# Supplementary material for: Deep Reinforcement Learning for Shared Autonomous Vehicles (SAV) Fleet Management
Source: arXiv:2201.05720 source file (2022-01-15)
Supplement: Supplementary file 1 [file appendix.tex]

\section{Overflow form other sections}
\label{sec:set-diff-dodis}

%%% Local Variables:
%%% mode: latex
%%% TeX-master: "main"
%%% End:
